# Supplementary material for: Magnon transport in $\mathrm{\mathbf{Y_3Fe_5O_{12}}}$/Pt nanostructures with reduced effective magnetization
Source: arXiv:2108.03263 ancillary file (2021-08-06)
Supplement: Supplementary file 1 [file SI_Magnon_transport_in_YIG-Pt_nanostructures_with_reduced_effective_magnetization.pdf]

# Supplemental Material: Magnon transport in $Y_3Fe_5O_{12}$/Pt nanostructures with reduced effective magnetization

J. Gückelhorn,[1,2,*] T. Wimmer,[1,2] M. Müller,[1,2] S. Geprägs,[1]
H. Huebl,[1,2,3] R. Gross,[1,2,3] and M. Althammer[1,2,†]

[1] *Walther-Meißner-Institut, Bayerische Akademie der Wissenschaften, 85748 Garching, Germany*

[2] *Physik-Department, Technische Universität München, 85748 Garching, Germany*

[3] *Munich Center for Quantum Science and Technology (MCQST), D-80799 München, Germany*

(Dated: July 20, 2021)

# I. YIG THIN FILMS ON YSGG

The 12.3 nm thick, single crystalline (111)-oriented yttrium iron garnet ($Y_3Fe_5O_{12}$, YIG) film was grown via pulsed laser deposition on an yttrium scandium gallium garnet ($Y_3Sc_2Ga_3O_{12}$, YSGG) substrate. A substrate temperature of 450 °C, an oxygen pressure of 25 µbar, a laser fluence at the target of 2.0 J/cm$^2$ and a laser frequency of 10 Hz were used.

For the broadband FMR experiments, a bare unpatterned YIG thin film is mounted on a coplanar waveguide utilized to measure the complex microwave transmission parameter $S_{21}$ via a vector network analyzer as a function of the applied microwave frequency and the magnetic field, which is applied in out-of-plane direction. From this data, we extracted the resonance field $\mu_0 H_{\mathrm{res}}$ and the linewidths $\mu_0 \Delta H$ as presented in the main text.

Furthermore, we performed SQUID (superconducting quantum interference device) magnetometry measurements to obtain the saturation magnetization $M_{\mathrm{s}}$, which is included as a fixed parameter in the calculation of the critical current dependence (see Sec. III). In this case, a 9 nm-thick YIG thin film grown on YSGG under the same conditions as the sample studied in the main text is utilized. The obtained magnetization $M$ is shown as a function of the in-plane magnetic field in Fig. S1 for a temperature of 300 K. Note that a linear (diamagnetic) background was subtracted from the data. We find a saturation magnetization

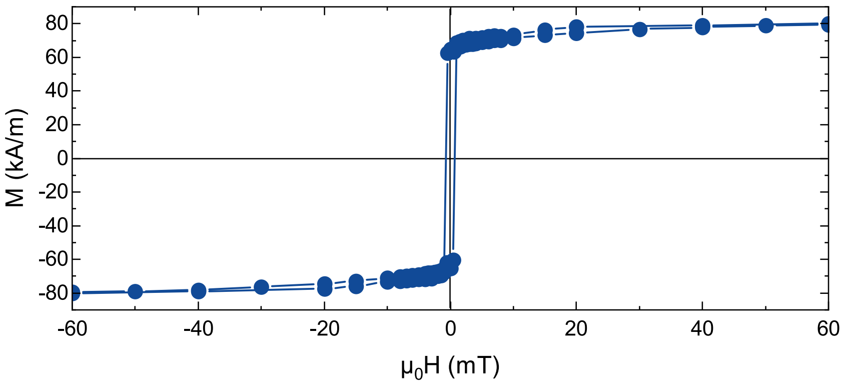


FIG. S1. In-plane SQUID magnetometry measurements of a 9 nm-thick YIG thin film grown on (111)-oriented YSGG at a temperature of 300 K. We observe a saturation magnetization $M_{\mathrm{s}} = 80\,\mathrm{kAm^{-1}}$.


* janine.gueckelhorn@wmi.badw.de

† matthias.althammer@wmi.badw.de

of $M_s = 80\,\mathrm{kAm^{-1}}$, which is smaller than the value observed for YIG thin films grown on lattice-matched GGG [S1].

## II. ALL-ELECTRICAL MAGNON TRANSPORT MEASUREMENTS

For an all-electrical generation and detection of pure spin currents 5 nm Pt was deposited on the YIG thin film using DC sputtering and strips were patterned into the films via e-beam lithography and lift-off. In a further patterning step, Al leads and bondpads were deposited to connect the device electrically. All measurements are conducted at $T = 280\,\mathrm{K}$, in accordance with our previous reports [S1, S2] to allow a better comparison.

For the twin-strip structure experiments (see Fig. 2(a) in the main text), we utilize the dc-detection technique. Here, a DC charge current $I^{\mathrm{inj}} = 100\,\mu\mathrm{A}$ is applied to the injector using a Keithley 2400 Sourcemeter and a Keithley 2182 Nanovoltmeter is used to detect the magnon transport signal at the detector. Using a current reversal technique, we can define the voltage due to SHE-induced magnons transported from the injector to the detector as

$$V_{\mathrm{SHE}}^{\mathrm{det}} = \frac{1}{2}\left[V^{\mathrm{det}}\left(I^{\mathrm{inj}}\right) - V^{\mathrm{det}}\left(-I^{\mathrm{inj}}\right)\right] \,. \tag{S1}$$

For the three-strip structure experiments (cf. Fig. 3(a) in the main text), the AC-readout technique was applied. In our previous work [S2], we have demonstrated that the data obtained by DC- and AC-detection techniques provide the same results, in particular for $I_{\mathrm{dc}}^{\mathrm{mod}} = 0\,\mathrm{A}$. Here, we used a Keithley 6221 current source to feed a low frequency ($f = 7.737\,\mathrm{Hz}$) AC charge current with a peak amplitude of $200\,\mu\mathrm{A}$ through the injector. The measured voltage signal at the detector is preamplified by a Standford Research System SR560 low-noise voltage amplifier before being passed to a Zurich Instruments HF2LI lock-in amplifier. Furthermore, the DC charge current $I_{\mathrm{dc}}^{\mathrm{mod}}$ applied to the modulator to manipulate the magnon transport is varied using a Keithley 2400 Sourcemeter. While the injector and detector width is kept constant at $w_{\mathrm{inj}} = w_{\mathrm{det}} = 500\,\mathrm{nm}$, the width of the modulator and the edge-to-edge distance between the strips varies. The injector and detector strips have a length $l = 50\,\mu\mathrm{m}$ and the modulator strip is $l = 64\,\mu\mathrm{m}$ long.

## III. CRITICAL CURRENT BEHAVIOR IN THE LIMIT OF VANISHING EFFECTIVE MAGNETIZATION

In this section, we discuss the dependence of the critical current on the applied magnetic field and material parameters such as the saturation magnetization $M_\mathrm{s}$ and derive the equation utilized in the main text. Please note that the discussion of this section is based on the theory of our previous work where we discussed the critical current dependence in the scope of damping compensation [S1].

In the regime of zero-effective damping, the magnon relaxation rate $\Gamma_\mathrm{mr}$ and anti-damping spin torque rate $\Gamma_\mathrm{ST}$ due to SHE have to compensate. Starting with $\Gamma_\mathrm{mr}$ of the lowest energy mode ($k = 0$), we find for an in-plane magnetized film

$$\Gamma_\mathrm{mr}^\mathrm{ip} = (\alpha_\mathrm{G} + \alpha_\mathrm{sp})\,\gamma\mu_0\left(H + \frac{M_\mathrm{eff}}{2}\right) \tag{S2}$$

with $\alpha_\mathrm{G}$ the Gilbert damping, $\alpha_\mathrm{sp}$ the Gilbert damping induced by spin pumping due to the adjacent heavy metal layer, $\gamma$ the gyromagnetic ratio, $\mu_0$ the Bohr magneton, $H$ the external field and $M_\mathrm{eff}$ the effective magnetization [S3]. The magnon relaxation rate is identical to the frequency linewidth of the $k = 0$ ferromagnetic resonance mode, which is given by

$$\Delta f = \Delta H\left(\frac{\partial\omega_\mathrm{FMR}(H)}{\partial H}\right)\,. \tag{S3}$$

where $\Delta H$ is the resonance linewidth, in our case extracted from broadband FMR measurements. In our experiments, we have to account for the FMR frequency

$$\omega_\mathrm{FMR}^\mathrm{ip}(H) = \gamma\mu_0\sqrt{H(H + M_\mathrm{eff})}, \tag{S4}$$

which is calculated from the Kittel formula for an in-plane magnetized film. Furthermore, inhomogeneous broadening $\delta H$ has to be considered and hence we introduce the effective damping parameter

$$\alpha_\mathrm{eff} = \alpha_\mathrm{G} + \gamma\mu_0\frac{\delta H}{2\omega_\mathrm{FMR}^\mathrm{ip}}, \tag{S5}$$

as demonstrated in Ref. [S4]. Substituting $\alpha_\mathrm{G}$ with $\alpha_\mathrm{eff}$ in Eq. (S2), we obtain

$$\Gamma_\mathrm{mr}^\mathrm{ip} = \left(\alpha_\mathrm{G} + \frac{\delta H}{2\sqrt{H(H + M_\mathrm{eff})}}\right)\gamma\mu_0\left(H + \frac{M_\mathrm{eff}}{2}\right) \tag{S6}$$

for the bare YIG thin film. Including inhomogenous broadening causes for finite $M_\mathrm{eff}$ a divergence of the damping rate $\Gamma_\mathrm{mr}^\mathrm{ip}$ for $H = 0$. However, in the limit of $M_\mathrm{eff} = 0$ we obtain

$$\Gamma_\mathrm{mr}^\mathrm{ip} = \gamma\mu_0\left(\alpha_\mathrm{G} H + \frac{\delta H}{2}\right)\,, \tag{S7}$$

which exhibits a constant magnon relaxation rate for $H = 0$. In addition, we obtain a strictly linear dependence on the magnetic field for $\Gamma_{\mathrm{mr}}^{\mathrm{ip}}$. As already discussed in the main text, we can utilize Eq. (S7) to describe the magnetic field dependence of the magnon diffusion length $\lambda_{\mathrm{m}}$ extracted from our all-electrical transport measurements. With $\lambda_{\mathrm{m}} = \sqrt{D\tau_{\mathrm{m}}}$, where $D$ corresponds to the magnon diffusion constant and $\tau_{\mathrm{m}}$ to the magnon lifetime, which can be calculated via $\tau_{\mathrm{m}} = {\Gamma_{\mathrm{mr}}^{\mathrm{ip}}}^{-1}$, we obtain the following equation

$$\lambda_{\mathrm{m}} = \sqrt{\frac{D}{\gamma\mu_0\left(\alpha_{\mathrm{G}}H + \frac{\delta H}{2}\right)}}\,. \tag{S8}$$

This expression is used in the main text as fitting function to determine $D$.

For the damping compensation, we need to again account for the interface injection rate via the spin Hall effect (SHE). The anti-damping spin torque rate in the macrospin approximation is given by [S4]

$$\Gamma_{\mathrm{ST}} = \frac{\hbar}{2e}\frac{\gamma}{M_{\mathrm{s}}t_{\mathrm{YIG}}t_{\mathrm{Pt}}w_{\mathrm{mod}}} \cdot T \cdot \theta_{\mathrm{SH}} I_{\mathrm{dc}}^{\mathrm{mod}}. \tag{S9}$$

Here, $M_{\mathrm{s}}$ is the saturation magnetization (determined via magnetometry measurements), $t_{\mathrm{YIG}}$ the thickness of the YIG film, $t_{\mathrm{Pt}}$ and $w_{\mathrm{mod}}$ are the thickness and the width of the modulator electrode, respectively, and $\theta_{SH}$ is the spin Hall angle of Pt. Moreover, $T$ denotes the interface spin transparency, which is given by

$$T = \frac{g^{\uparrow\downarrow}\tanh(\eta)}{g^{\uparrow\downarrow}\coth(2\eta) + \frac{h}{2e^2}\frac{\sigma_{\mathrm{Pt}}}{l_{\mathrm{s}}}} \tag{S10}$$

where $\eta = \frac{t_{\mathrm{Pt}}}{2l_{\mathrm{s}}}$ with the spin diffusion length $l_{\mathrm{s}}$ of Pt, $\sigma_{\mathrm{Pt}}$ the electrical conductivity of Pt and $g^{\uparrow\downarrow}$ the interface spin mixing conductance [S5]. Note, that we approximate $\coth(2\eta) \approx 1$ in Eq. (S10), since the thickness $t_{\mathrm{Pt}}$ of our Pt thin film is larger than $2l_{\mathrm{s}}$. Now, we have to account for the spin pumping contribution to the damping $\alpha_{\mathrm{sp}}$ for the magnon relaxation rate $\Gamma_{\mathrm{mr}}^{\mathrm{ip}}$ due to the Pt modulator interface. The Gilbert damping induced by spin pumping is given by

$$\alpha_{\mathrm{sp}} = g_{\mathrm{eff}}\frac{\hbar\gamma}{4\pi M_{\mathrm{s}}t_{\mathrm{YIG}}} \tag{S11}$$

with the effective spin mixing conductance

$$g_{\mathrm{eff}} = \frac{g^{\uparrow\downarrow}\frac{h}{2e^2}\frac{\sigma_{\mathrm{Pt}}}{l_{\mathrm{s}}}}{g^{\uparrow\downarrow} + \frac{h}{2e^2}\frac{\sigma_{\mathrm{Pt}}}{l_{\mathrm{s}}}} \tag{S12}$$

| | Symbol | Value | Unit |
|---|---|---|---|
| Pt strip thickness | $\mathrm{t_{Pt}}$ | 5 | nm |
| Pt spin diffusion length [S7] | $\mathrm{l_s}$ | 1.5 | nm |
| Pt spin Hall angle [S7] | $\theta_{\mathrm{SH}}$ | 0.11 | |
| YIG thickness | $\mathrm{t_{YIG}}$ | 12.3 | nm |
| gyromagnetic ratio | $\gamma$ | $1.76 \times 10^{11}$ | rad/Ts |
| YIG saturation magnetization | $M_{\mathrm{s}}$ | 80 | $\mathrm{kAm^{-1}}$ |
| inhomogeneous broadening | $\mu_0\delta\mathrm{H}$ | 3.6 | mT |
| Gilbert damping | $\alpha_{\mathrm{G}}$ | $1.5 \times 10^{-3}$ | |
| YIG effective magnetization | $\mu_0 M_{\mathrm{eff}}$ | 56 | mT |

TABLE S1. Values for the parameters used for the fitting curves in Fig. S2.

to account for the finite interface transparency. In the following, we utilize for the magnon relaxation

$$\Gamma_{\mathrm{mr}}^{\mathrm{ip}} = \left(\alpha_{\mathrm{sp}} + \alpha_{\mathrm{G}} + \frac{\delta H}{2\sqrt{H\left(H + M_{\mathrm{eff}}\right)}}\right)\gamma\mu_0\left(H + \frac{M_{\mathrm{eff}}}{2}\right) \ . \tag{S13}$$

When the condition $\Gamma_{\mathrm{mr}}^{\mathrm{ip}} = \Gamma_{\mathrm{ST}}$ is met, a coherent precession of the magnetization with zero effective damping is present and we can define the critical current $I_{\mathrm{crit}}^{\mathrm{mod}}$ by equating Eqs. (S13) and (S9):

$$I_{\mathrm{crit}}^{\mathrm{mod}} = \frac{2e}{\hbar}\frac{M_{\mathrm{s}}t_{\mathrm{YIG}}}{\gamma}\frac{t_{\mathrm{Pt}}w_{\mathrm{mod}}}{T\theta_{\mathrm{SH}}}\left(\alpha_{\mathrm{sp}} + \alpha_{\mathrm{G}} + \frac{\delta H}{2\sqrt{H\left(H + M_{\mathrm{eff}}\right)}}\right)\gamma\mu_0\left(H + \frac{M_{\mathrm{eff}}}{2}\right) \ . \tag{S14}$$

Utilizing Eqs. (S10) and (S12), we can rewrite this expression and obtain

$$I_{\mathrm{crit}}^{\mathrm{mod}} = \frac{\hbar}{e}\frac{\sigma_{\mathrm{Pt}}}{2l_{\mathrm{s}}}\frac{t_{\mathrm{Pt}}w_{\mathrm{mod}}}{\theta_{\mathrm{SH}}\tanh(\eta)}\left(1 + 4\pi M_{\mathrm{s}}t_{\mathrm{YIG}}\frac{\alpha_{\mathrm{eff}}}{\hbar\gamma g_{\mathrm{eff}}}\right)\gamma\mu_0\left(H + \frac{M_{\mathrm{eff}}}{2}\right) \ , \tag{S15}$$

which is the same result as already obtained in our previous work [S1]. As discussed in the main text, we can now look into the limit $M_{\mathrm{eff}} = 0$, which lifts the divergence for $H = 0$, obtaining

$$I_{\mathrm{crit}}^{\mathrm{mod}} = \frac{\hbar}{e}\frac{\sigma_{\mathrm{Pt}}}{2l_{\mathrm{s}}}\frac{t_{\mathrm{Pt}}w_{\mathrm{mod}}}{\theta_{\mathrm{SH}}\tanh(\eta)}\left(\mu_0 H\left[\gamma + 4\pi M_{\mathrm{s}}t_{\mathrm{YIG}}\frac{\alpha_{\mathrm{G}}}{\hbar g_{\mathrm{eff}}}\right] + 4\pi M_{\mathrm{s}}t_{\mathrm{YIG}}\frac{\mu_0\frac{\delta H}{2}}{\hbar g_{\mathrm{eff}}}\right) \ . \tag{S16}$$

We obtain a linear dependence on the external magnetic field in accordance with the results by Evelt *et al.* in Bi:YIG thin films [S6]. As already presented in the main text, we

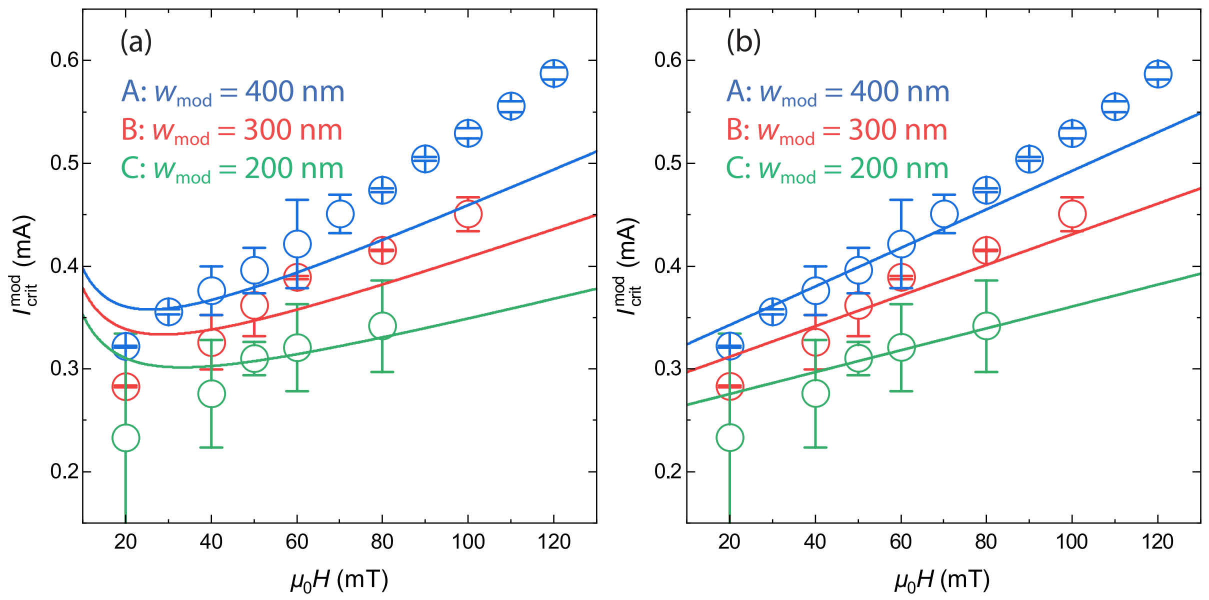


FIG. S2. Extracted critical currents $I_{\mathrm{crit}}^{\mathrm{mod}}$ as a function of the magnetic field magnitude $\mu_0 H$ for device A (blue data points) presented in the main text and additional data of the devices B and C (red and green data points, respectively). (a) The critical current dependence is fitted to Eq. (S15). (b) The data is fitted in the limit of vanishing effective magnetization ($M_{\mathrm{eff}} = 0$) by Eq. (S16).

| Symbol | unit | Device A | Device B | Device C |
|---|---|---|---|---|
| $w_{\mathrm{mod}}$ | nm | 400 | 300 | 200 |
| $\sigma_{\mathrm{Pt}}$ | $10^6(\Omega\mathrm{m})^{-1}$ | 2.15 | 2.22 | 2.26 |
| $g^{\uparrow\downarrow}$ | $10^{18}\mathrm{m}^{-2}$ | $17 \pm 2$ | $11 \pm 1$ | $6.5 \pm 0.2$ |
| $g^{\uparrow\downarrow}$ ($M_{\mathrm{eff}} = 0$) | $10^{18}\mathrm{m}^{-2}$ | $9.9 \pm 0.4$ | $7.6 \pm 0.3$ | $5.2 \pm 0.1$ |

TABLE S2. Device dependent parameters and experimentally determined interface spin mixing conductance $g^{\uparrow\downarrow}$ extracted from fits in Fig. S2 to Eq. (S15) and Eq. (S16) in the limit $M_{\mathrm{eff}} = 0$.

can either utilize Eqs. (S15) or (S16) to describe the measured magnetic field dependence of the critical current. Here, we present the data for two more devices (device $B$ with $w_{\mathrm{mod}} = 300\,\mathrm{nm}$, device $C$ with $w_{\mathrm{mod}} = 200\,\mathrm{nm}$) on the same YIG thin film grown on YSGG. In Fig. S2, their critical current $I_{\mathrm{crit}}^{\mathrm{mod}}$ is plotted as a function of the magnetic filed magnitude $\mu_0 H$ and for comparison we also included the data of the structure investigated in the main text (device $A$ with $w_{\mathrm{mod}} = 400\,\mathrm{nm}$). The three structures exhibit an edge-to-edge distance of $d_{\mathrm{e}} = 200\,\mathrm{nm}$, while their modulator widths $w_{\mathrm{mod}}$ vary. To compare the two models, the

data is fitted by Eq. (S15) in Fig. S2(a) and by Eq. (S16) in Fig. S2(b). Again, the interface spin mixing conductance $g^{\uparrow\downarrow}$ is the only free fit parameter and the values used as fixed parameters in both cases can be found in Tab. S1. Our findings corroborate the results found in the main text: Accounting for the finite $M_{\text{eff}}$, we only observe a quantitatively good agreement for $\mu_0 H \geq 40\,\text{mT}$ (cf. Fig. S2(a)), while assuming $M_{\text{eff}} \approx 0$ describes our data quantitatively well over the whole magnetic field range shown here (cf. Fig. S2(b)). For both fits the obtained values of $g^{\uparrow\downarrow}$ are shown in Tab. S2. For both fitting functions, we obtain values similar to YIG/Pt structures on GGG [S1]. As already discussed in the main text, the deviations between fit and data can be attributed to uncertainties of the fixed parameters.

---


[S1] T. Wimmer, M. Althammer, L. Liensberger, N. Vlietstra, S. Geprägs, M. Weiler, R. Gross, and H. Huebl, Spin transport in a magnetic insulator with zero effective damping, Physical Review Letters **123**, 257201 (2019).

[S2] J. Gückelhorn, T. Wimmer, S. Geprägs, H. Huebl, R. Gross, and M. Althammer, Quantitative comparison of magnon transport experiments in three-terminal YIG/Pt nanostructures acquired via dc and ac detection techniques, Applied Physics Letters **117**, 182401 (2020).

[S3] B. Hillebrands and A. Thiaville, *Spin Dynamics in Confined Magnetic Structures III* (Springer, Berlin, Heidelberg, 2006).

[S4] M. Collet, X. De Milly, O. d. Kelly, V. V. Naletov, R. Bernard, P. Bortolotti, J. B. Youssef, V. Demidov, S. Demokritov, J. L. Prieto, M. Muñoz, V. Cros, A. Anane, G. de Loubens, and O. Klein, Generation of coherent spin-wave modes in yttrium iron garnet microdiscs by spin–orbit torque, Nature communications **7**, 10377 (2016).

[S5] W. Zhang, W. Han, X. Jiang, S.-H. Yang, and S. Parkin, Role of transparency of platinum-ferromagnet interface in determining intrinsic magnitude of spin hall effect, Nature Physics **11**, 496 (2015).

[S6] M. Evelt, L. Soumah, A. Rinkevich, S. Demokritov, A. Anane, V. Cros, J. Ben Youssef, G. de Loubens, O. Klein, P. Bortolotti, and V. Demidov, Emission of coherent propagating magnons by insulator-based spin-orbit-torque oscillators, Physical Review Applied **10**, 041002 (2018).

[S7] M. Althammer, S. Meyer, H. Nakayama, M. Schreier, S. Altmannshofer, M. Weiler, H. Huebl, S. Geprägs, M. Opel, R. Gross, D. Meier, C. Klewe, T. Kuschel, J.-M. Schmalhorst, G. Reiss, L. Shen, A. Gupta, Y.-T. Chen, G. E. W. Bauer, E. Saitoh, and S. T. B. Goennenwein, Quantitative study of the spin Hall magnetoresistance in ferromagnetic insulator/normal metal hybrids, Physical Review B **87**, 224401 (2013).
